# Supplementary material for: Resolving Geometric Excitations of Fractional Quantum Hall States
Source: arXiv:2406.11195 source file (2024-07-01)
Supplement: Supplementary file 1 [file Appendix.pdf]

# Supplemental Materials: Resolving Geometric Excitations of Fractional Quantum Hall States

Yang Liu,<sup>1,2</sup> Tong Zhou Zhao,<sup>1</sup> and T. Xiang<sup>1,2,\*</sup>

<sup>1</sup>*Beijing National Laboratory for Condensed Matter Physics and Institute of Physics,  
Chinese Academy of Sciences, Beijing 100190, China.*

<sup>2</sup>*School of Physical Sciences, University of Chinese Academy of Sciences, Beijing 100049, China.*

## Appendix A: Parent Hamiltonians of fractional quantum Hall states on a cylinder

In this section, we elucidate the formalism of the fractional quantum Hall effect (FQHE) on a cylinder. While the formalism used in our analysis is conventional, a thorough introduction to these aspects is beneficial, as published articles often omit crucial details. To enhance readability and ensure logical consistency, we will restate some equations previously mentioned in the main text.

The system under consideration is defined on an open cylinder aligned along the  $x$ -direction. The length and circumference of the cylinder are denoted as  $L_x$  and  $L_y$ , respectively. During subsequent infinite tensor network calculations, we take the limit  $L_x \rightarrow \infty$ . We utilize the Landau gauge  $\mathbf{A} = (0, Bx, 0)$  and consider only the orbitals in the lowest Landau level. The  $m$ th single-particle wave function in the lowest Landau level is defined as:

$$\phi_m(x, y) = \frac{1}{\sqrt{\pi^{1/2} L_y}} e^{ime_y l y} e^{-(x-me_y l)^2/2} \quad (\text{A1})$$

where  $e_y = 2\pi/L_y$  and  $l = \sqrt{\hbar c/eB}$  is the magnetic length. In the discussion below, we set below  $l = 1$ . This Landau orbital has well-defined momentum  $k = (k_x, k_y)$  on an infinite cylinder. The momentum along the  $y$ -axis is quantized  $k_y = me_y$ , while that along the  $x$ -axis is continuous.

A generic two-body interaction in the momentum space reads

$$v(r_1 - r_2) = \sum_k v_k e^{ik \cdot (r_1 - r_2)}. \quad (\text{A2})$$

By utilizing the formula

$$\langle \phi_{m_1} \phi_{m_2} | e^{ik \cdot (r_1 - r_2)} | \phi_{n_1} \phi_{n_2} \rangle = \langle \phi_{m_1} | e^{ik \cdot r_1} | \phi_{n_1} \rangle \langle \phi_{m_2} | e^{-ik \cdot r_2} | \phi_{n_2} \rangle, \quad (\text{A3})$$

$$\langle \phi_m | e^{ik \cdot r} | \phi_n \rangle = \delta_{(m-n)e_y, k_y} e^{-\frac{k^2}{4} + i\frac{k_x k_y}{2} + i n k_x e_y}, \quad (\text{A4})$$

we can further express this two-body interaction, also called the parent Hamiltonian, as

$$H = \sum_{k_x} \sum_m v_k \left( e^{-\frac{1}{4} k^2} \rho_{k_x, me_y} \right) \left( e^{-\frac{1}{4} k^2} \rho_{-k_x, -me_y} \right) = \sum_k V_k \rho_k \rho_{-k} \quad (\text{A5})$$

where  $\rho_k$  is the projected density operator

$$\rho_k = \rho_{k_x, me_y} = \sum_n \exp \left[ \frac{i \tilde{k}_x (2n + m)}{2} \right] c_n^\dagger c_{n+m}, \quad (\text{A6})$$

$\tilde{k}_x = k_x e_y$ , and  $c_m^\dagger$  the creation operator of electron.  $V_k = [F(k)]^2 v_k$  is the Fourier transform of the projected interaction, and  $F(k) = \exp(-k^2/4)$  is the form factor for the lowest Landau level.

The Fourier transform of the  $V_1$ -Haldane pseudopotential or Trugman-Kivelson real space potential  $\nabla_i^2 \delta^2(r_i - r_j)$  is  $v_k = 1 - k^2$  [1, 2]. It corresponds to the zero energy Laughlin state. Substituting this expression into Eq. (A5), we find the parent Hamiltonian of the Laughlin state to be:

$$H_L = \frac{(2\pi)^{5/2}}{L_y^3} \sum_{j_1 j_2 j_3 j_4} (j_1 - j_2) (j_3 - j_4) e^{-e_y^2 [(j_1 - j_4)^2 + (j_2 - j_3)^2]/2} \delta_{j_1 + j_2, j_3 + j_4} c_{j_1}^\dagger c_{j_2}^\dagger c_{j_3} c_{j_4} \quad (\text{A7})$$

---

\* txiang@iphy.ac.cn

The three-body Hamiltonian for the Moore-Read (MR) state can be similarly derived. The result is

$$H_{\text{MR}} = \sum_{k_1, k_2} V_{k_1, k_2} \rho_{k_1} \rho_{k_2} \rho_{-k_1 - k_2}, \quad (\text{A8})$$

where

$$V_{k_1, k_2} = F(k_1)F(k_2)F(-k_1 - k_2)v(k_1, k_1), \quad (\text{A9})$$

and  $v(k_1, k_1)$  is the Fourier transform of the three-body interaction

$$\nabla_i^4 \nabla_j^2 \delta^2(r_i - r_j) \delta^2(r_j - r_k), \quad (\text{A10})$$

which reads

$$v(k_1, k_1) = k_1^4 k_2^2 + k_1^2 k_2^4 + k_2^4 (k_1 + k_2)^2 + k_2^2 (k_1 + k_2)^4 + k_1^4 (k_1 + k_2)^2 + k_1^2 (k_1 + k_2)^4. \quad (\text{A11})$$

$H_{\text{MR}}$  can also be expressed as [3, 4]

$$H_{\text{MR}} = \frac{1024\sqrt{3}\pi^7}{L_y^8} \sum_{j_1, j_2, j_3, j_4, j_5, j_6} (j_1 - j_2)(j_1 - j_3)(j_2 - j_3)(j_6 - j_4)(j_6 - j_5)(j_5 - j_4) \delta_{j_1 + j_2 + j_3, j_4 + j_5 + j_6} \exp \left\{ -\frac{2\pi^2}{L_y^2} \left[ \sum_i j_i^2 - \frac{1}{6} \left( \sum_i j_i \right)^2 \right] \right\} c_{j_1}^\dagger c_{j_2}^\dagger c_{j_3}^\dagger c_{j_4} c_{j_5} c_{j_6} \quad (\text{A12})$$

## Appendix B: MPS representation of the ground state

For a translation invariant system, the MPS of the ground state reads

$$\Psi = \dots - \textcircled{A} - \textcircled{A} - \textcircled{A} - \dots, \quad (\text{B1})$$

where  $A$  is the local tensor defined for a unit cell. If this unit cell contains  $M$  sites, we further decompose  $A$  as a product of  $M$  local tensors defined on each site by  $A_l (l = 1, \dots, M)$ .

The Laughlin ground states are three-fold topological degenerate, corresponding to the following three initial orbital configurations (or the root partitions [5–7]):  $\{\dots 100100\dots\}$ ,  $\{\dots 010010\dots\}$ , and  $\{\dots 001001\dots\}$ . Thus, we can set  $M = 3$  and represent  $A$  as

$$\textcircled{A} = \textcircled{A_1} \textcircled{A_2} \textcircled{A_3} \quad (\text{B2})$$

The Laughlin state conserves the particle number and the  $y$ -axis momentum on a cylinder [8, 9]. Thus, we can assign both the particle number  $C_l$  and the momentum  $K_l$  to the vertical leg of local tensor  $A_l$ . For a given filling factor  $\nu$ ,  $(K_l, C_l)$  are defined by [8–10]

$$K_l = l(N_l - \nu), \quad (\text{Momentum}) \quad (\text{B3})$$

$$C_l = N_l - \nu, \quad (\text{Particle number}) \quad (\text{B4})$$

where  $N_l$  is the particle number at site  $l$ . Similarly, we can introduce the corresponding quantum numbers  $(\bar{K}, \bar{C})$  for each horizontal bond.

Under a translation by  $M$  sites, the physical and virtual momenta,  $K_l$  and  $\bar{K}_l$ , behave as

$$K_l \rightarrow K_l + MC_l, \quad (\text{B5})$$

$$\bar{K}_l \rightarrow \bar{K}_l + M\bar{C}_l. \quad (\text{B6})$$

This property should be taken into account in the implementation of the DMRG algorithm [9, 11, 12] and in the translation of MPS with a periodicity  $M$ .

For each local tensor, the quantum numbers satisfy the following addition rule:

$$(\bar{K}, \bar{C})_{l,\text{left}} + (K_l, C_l) - (\bar{K}, \bar{C})_{l,\text{right}} = 0 \quad (\text{B7})$$

A similar idea works for the Moore-Read (MR) state. In the even parity state, we can choose the orbital configuration  $\{\dots 10011001\dots\}$  to represent the ground state. This indicates that the minimum cell of the ground state is  $M = 4$  and

$$\text{---} \bigcirc \! \! \! \overset{|}{A} \text{---} = \text{---} \bigcirc \! \! \! \overset{|}{A_1} \text{---} \bigcirc \! \! \! \overset{|}{A_2} \text{---} \bigcirc \! \! \! \overset{|}{A_3} \text{---} \bigcirc \! \! \! \overset{|}{A_4} \text{---} . \quad (\text{B8})$$

In the odd-parity sector of the MR state, there are unpaired fermions. In this case, the initial orbital configuration changes from  $\{\dots 1001\dots\}$  to  $\{\dots 01\dots\}$ , and the corresponding unit cell changes from 4 to 2. Thus,  $A$  can be represented as

$$\text{---} \bigcirc \! \! \! \overset{|}{A} \text{---} = \text{---} \bigcirc \! \! \! \overset{|}{A_1} \text{---} \bigcirc \! \! \! \overset{|}{A_2} \text{---} . \quad (\text{B9})$$

In addition, a one-half quantum flux  $f = 1/2$  should attach to a local tensor in each unit cell to correctly capture the topological nature of the neutral fermion mode. Accordingly, Eq. (B7) becomes

$$(\bar{K}, \bar{C})_{l,\text{left}} + (K_l + f, C_l) - (\bar{K}, \bar{C})_{l,\text{right}} = (0, 0) \quad (\text{B10})$$

We determine all local tensors by variationally minimizing the ground state energy using the standard tensor-network methods, including the density matrix renormalization group (DMRG) and variational uniform matrix product states (VUMPS) [13]. For benchmarking, we calculate the entanglement spectrum of both the Laughlin and MR states. As shown in Fig. 1, the entanglement spectrum patterns of these two states obtained from our calculation are consistent with the CFT.

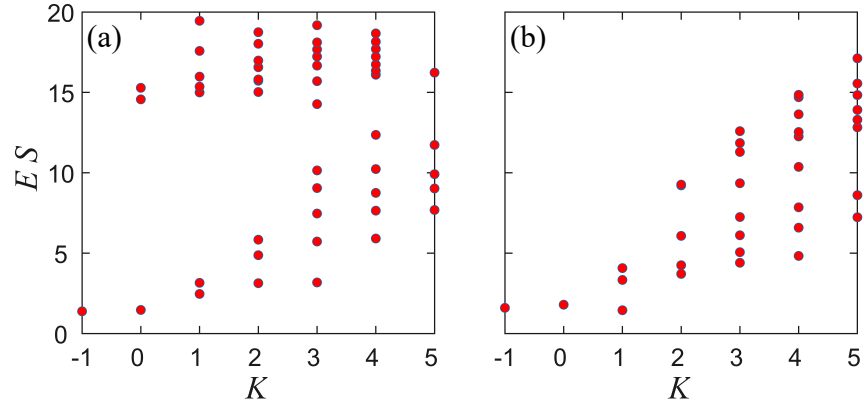

FIG. 1. Entanglement spectra of (a) the Laughlin state, the counting pattern is 1,1,2,3,5,..., and (b) the MR state, the counting pattern is 1,1,3,5,... [14].

### Appendix C: MPS representation of excited states under the single-mode approximation

Under the single-mode approximation, the excited states are represented by replacing one of the  $A$  tensors in the ground state with an impurity tensor  $B$  and then boosting into a momentum eigenstate

$$\Phi_k(B) = \sum_n e^{i\tilde{k}_x n M} \dots \text{---} \bigcirc \! \! \! \overset{|}{A} \text{---} \bigcirc \! \! \! \overset{|}{B} \text{---} \bigcirc \! \! \! \overset{|}{A} \text{---} \dots \quad (\text{C1})$$

In this expression,  $B$  is defined on one of the unit cells. Like  $A$ , it can be further decomposed as sum of  $M$  MPS

$$\text{---} \bigcirc \! \! \! \overset{|}{B} \text{---} = \text{---} \bigcirc \! \! \! \overset{|}{B_1} \text{---} \bigcirc \! \! \! \overset{|}{A_2} \text{---} \dots \text{---} \bigcirc \! \! \! \overset{|}{A_M} \text{---} + \dots + e^{i\tilde{k}_x (M-1)} \text{---} \bigcirc \! \! \! \overset{|}{A_1} \text{---} \bigcirc \! \! \! \overset{|}{A_2} \text{---} \dots \text{---} \bigcirc \! \! \! \overset{|}{B_M} \text{---} , \quad (\text{C2})$$

where  $\tilde{k}_x = e_y k_x$  and  $(B_1, \dots, B_M)$  are the local impurity tensors to be variationally determined. In the study of neutral fermions in the odd-parity sector of the MR state, as the unit cell is reduced from  $M = 4$  to 2, we should shift the central momentum from 0 to  $\pi$ , by setting  $\tilde{k}_x \rightarrow \tilde{k}_x \pm \frac{\pi}{2}$ .

It is simple to show that the above MPS is invariant under the following gauge transformation

$$B_l \rightarrow B_l + A_l X_l - e^{-ik} X_l A_l, \quad (\text{C3})$$

where  $X_l$  is an arbitrary bond matrix.

Clearly,  $\Phi_k(B)$  is orthogonal to the ground state,  $\langle \Psi(A) | \Phi_k(B) \rangle = 0$ , if  $k$  is finite. To ensure  $\Phi_k(B)$  orthogonal to the ground state even in the case  $k = 0$ ,  $B_l$  should also be orthogonal to  $A_l$  if  $(A_1, \dots, A_M)$  are left canonicalized, satisfying the constraint

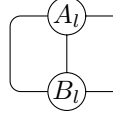

$$= 0. \quad (\text{C4})$$

In this case,  $B_l$  can be further parameterized as

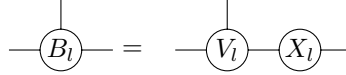

$$(\text{C5})$$

where  $V_l$  is the null-space tensor of  $A_l$  and  $X_l$  is variational bond matrix determined by the equation [15]

$$H_k^{\text{eff}} X = E_k X, \quad (\text{C6})$$

where  $H_k^{\text{eff}}$  is the effective Hamiltonian determined by the derivative

$$H_k^{\text{eff}} = \frac{\delta^2}{\delta(X')^\dagger \delta X} \langle \Phi_k(B') | H | \Phi_k(B) \rangle, \quad (\text{C7})$$

where  $X = (X_1, \dots, X_M)$ .

For details on the evaluation of the effective Hamiltonian  $H^{\text{eff}}$ , we refer readers to Ref. [16].

#### Appendix D: Static structure factor

In Fig. 1 of the main text, we show the static structure factor  $S(k)$  along the  $k_x$  direction with  $k_y = 0$ . Here, we provide more information on this static structure factor for the Laughlin and MR states. Figure 2 shows the density plot of  $S(k)$  on the whole  $(k_x, k_y)$  plane. Our calculation indicates that  $S(k)$  is isotropic. The peak (high intensity) positions of  $S(k)$  are consistent with previous studies [17].

- 
- [1] F. D. M. Haldane, Fractional quantization of the hall effect: A hierarchy of incompressible quantum fluid states, [Phys. Rev. Lett. \*\*51\*\*, 605 \(1983\)](#).
  - [2] S. A. Trugman and S. Kivelson, Exact results for the fractional quantum Hall effect with general interactions, [Phys. Rev. B \*\*31\*\*, 5280 \(1985\)](#).
  - [3] A. Kirmani, K. Bull, C.-Y. Hou, V. Saravanan, S. M. Saeed, Z. Papić, A. Rahmani, and P. Ghaemi, Probing geometric excitations of fractional quantum hall states on quantum computers, [Phys. Rev. Lett. \*\*129\*\*, 056801 \(2022\)](#).
  - [4] C. Voinea, S. Pu, A. Kirmani, P. Ghaemi, A. Rahmani, and Z. Papić, Deformed fredkin model for the  $\nu = 5/2$  moore-read state on thin cylinders, [Phys. Rev. Res. \*\*6\*\*, 013105 \(2024\)](#).
  - [5] B. A. Bernevig and F. D. M. Haldane, Generalized clustering conditions of jack polynomials at negative jack parameter  $\alpha$ , [Phys. Rev. B \*\*77\*\*, 184502 \(2008\)](#).
  - [6] B. A. Bernevig and F. D. M. Haldane, Model fractional quantum hall states and jack polynomials, [Phys. Rev. Lett. \*\*100\*\*, 246802 \(2008\)](#).
  - [7] B. Yang, Z.-X. Hu, Z. Papić, and F. D. M. Haldane, Model wave functions for the collective modes and the magnetoroton theory of the fractional quantum hall effect, [Phys. Rev. Lett. \*\*108\*\*, 256807 \(2012\)](#).
  - [8] M. P. Zaletel and R. S. K. Mong, Exact matrix product states for quantum hall wave functions, [Phys. Rev. B \*\*86\*\*, 245305 \(2012\)](#).

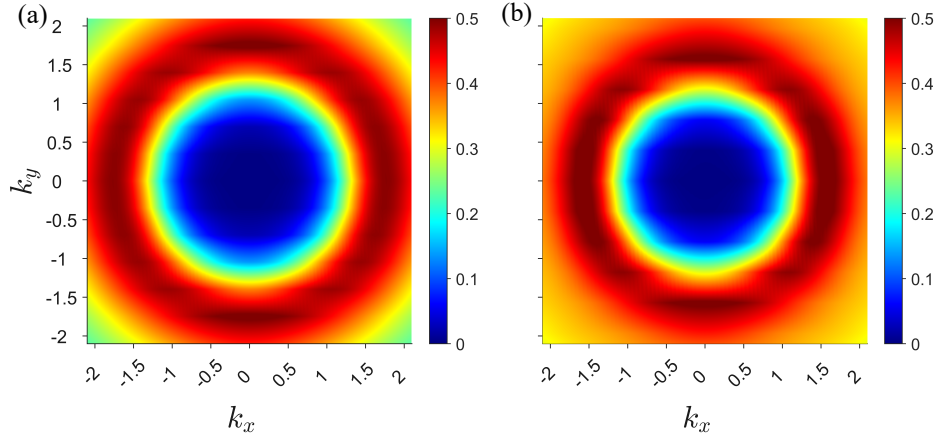

FIG. 2. Density plot of the static structure factor  $S(k)$  defined in Eq. (7) of the main text in the  $(k_x, k_y)$  plane for (a) the Laughlin state with  $L_y = 18$  and (b) the MR state with  $L_y = 16$ .

- [9] M. P. Zaletel, R. S. K. Mong, and F. Pollmann, Topological characterization of fractional quantum hall ground states from microscopic hamiltonians, *Phys. Rev. Lett.* **110**, 236801 (2013).
- [10] L. Hu and W. Zhu, Abelian origin of  $\nu = 2/3$  and  $2 + 2/3$  fractional quantum hall effect, *Phys. Rev. B* **105**, 165145 (2022).
- [11] S. R. White, Density matrix formulation for quantum renormalization groups, *Phys. Rev. Lett.* **69**, 2863 (1992).
- [12] S. R. White, Density-matrix algorithms for quantum renormalization groups, *Phys. Rev. B* **48**, 10345 (1993).
- [13] V. Zauner-Stauber, L. Vanderstraeten, M. T. Fishman, F. Verstraete, and J. Haegeman, Variational optimization algorithms for uniform matrix product states, *Phys. Rev. B* **97**, 045145 (2018).
- [14] H. Li and F. D. M. Haldane, Entanglement spectrum as a generalization of entanglement entropy: Identification of topological order in non-abelian fractional quantum hall effect states, *Phys. Rev. Lett.* **101**, 010504 (2008).
- [15] L. Vanderstraeten, J. Haegeman, and F. Verstraete, Tangent-space methods for uniform matrix product states, *SciPost Phys. Lect. Notes*, **7** (2019).
- [16] T. Xiang, *Density matrix and tensor network renormalization* (Cambridge University Press, 2023).
- [17] J. Wang, S. D. Geraedts, E. H. Rezayi, and F. D. M. Haldane, Lattice monte carlo for quantum hall states on a torus, *Phys. Rev. B* **99**, 125123 (2019).
